# Supplementary material for: GeoAuxNet: Towards Universal 3D Representation Learning for Multi-sensor Point Clouds
Source: arXiv:2403.19220 source file (2024-03-28)
Supplement: Supplementary file 1 [file X_suppl.tex]

\clearpage
\maketitlesupplementary

\section{Additional Experiments}

\subsection{Experiment Settings}
\noindent\textbf{Training Methodology.} The comprehensive configuration for the joint pre-training and subsequent fine-tuning phases is shown in Table~\ref{tab:implementation details}. The GeoAuxNet model is subjected to joint pre-training utilizing three distinct datasets: S3DIS~\cite{S3DIS2016CVPR} and ScanNet~\cite{ScanNet2017CVPR} derived from RGB-D camera, and SemanticKITTI~\cite{SemanticKITTI2019ICCV} obtained via LiDAR. To account for variations in dataset scale, we established a sampling ratio of 2:2:5 across these datasets. Subsequently, the pre-trained GeoAuxNet model undergoes fine-tuning on each dataset independently, employing a reduced learning rate. The total number of training iterations is equal to the sum of the best performance necessary iteration numbers for all three datasets.
\begin{table}[h]
    \centering
    \caption{Detailed training settings of semantic segmentation experiments.}
    \begin{tabular}{l|c}
    \toprule
    Config        & Pre-training     \\ \midrule
    optimizer     & SGD              \\
    scheduler     & OneCycleLR       \\
    learning rate & 0.05             \\
    weight decay  & $10^{-4}$        \\
    momentum      & 0.9              \\
    batch size    & 24               \\
    epoch         & 100              \\
    \bottomrule
    \end{tabular}
    
    \label{tab:implementation details}
\end{table}

\noindent\textbf{Network Architectures.} The detailed information of our backbone and point network is outlined in Table~\ref{tab:network architecture}. The point network only contains 1.1M parameters which can be ignored compared with the voxel backbone. But it improves the performance by about 6\% in mIoU on three datasets, as illustrated in Table~\ref{tab:voxel backbone results}.

\begin{table}[h]
    \centering
    \caption{Details of the network architectures in GeoAuxNet.}
    
    \resizebox{\linewidth}{!}{\begin{tabular}{l|cc}
    \toprule
    Config                  & Voxel backbone                          & Point network               \\ \midrule
    embedding channels      & 32                                      & 32                          \\
    encoder layers          & [2, 3, 4, 6]                            & [2, 2, 2, 2]                \\
    encoder channels        & [32, 64, 128, 256]                      & [32, 64, 128, 256]          \\ 
    decoder layers          & [2, 2, 2, 2]                            & [2, 2, 2, 2]                \\ 
    decoder channels        & [256, 128, 96, 96]                      & [256, 128, 96, 96]          \\ \bottomrule
    \end{tabular}
    }
    \label{tab:network architecture}
\end{table}

\begin{table}[h]
    \centering
    \caption{Semantic segmentation results on three benchmarks. We train the voxel backbone and GeoAuxNet on the joint training data of three datasets. We report the mIoU (\%) on Area 5 of S3DIS and validation sets of ScanNet and SemanticKITTI.}
    \small
    \resizebox{\linewidth}{!}{\begin{tabular}{l|lll}
    \toprule
    Methods    & S3DIS      & ScanNet     & SemanticKITTI \\ \midrule
    Voxel backbone   &     $63.4$&     $64.7$&    $57.9$\\ 
    GeoAuxNet        & $69.5_{\textcolor{Green}{(+6.1)}}$& $71.3_{\textcolor{Green}{(+6.6)}}$ & $63.8_{\textcolor{Green}{(+·5.9)}}$\\ \bottomrule
    \end{tabular}
    }
    
    \label{tab:voxel backbone results}
\end{table}

\subsection{Additional Results}

We further conduct experiments with different training datasets. As shown in Table~\ref{tab:additional results}, the observed improvements are consistent on different selections of datasets.

% \noindent\textbf{Original PPT.} The original PPT model is trained using language-guided categorical alignment on the joint training datasets. The results on S3DIS, ScanNet and SemanticKITTI are presented in Table~\ref{tab:additional results}.
% Due to the diversity of categorical labels of point clouds from RGB-D cameras and LiDAR, language-guided alignment fails to converge on the joint training data. The absence of decoupled projection heads and a limited number of parameters contribute to a diminished general representation capability across point clouds from different sensors.

% \noindent\textbf{MinkowskiNet.} 
% We train MinkowskiNet~\cite{SparseUNet2019CVPR} with decoupled projection heads on three datasets simultaneously. Without dataset-aware batch normalization introduced in previous works~\cite{PPT2023ArXiv, CDCL2021AAAI}, the domain gap across datasets limits MinkowskiNet in extracting sensor-specific features during training.
\begin{table}[h]
    \centering
    \caption{Semantic segmentation results on different selections of training datasets. The yellow columns stand for the results of three methods trained on S3DIS and nuScenes collectively, while the blue columns are the results of training on ScanNet and nuScenes.  We report the mIoU (\%) on Area 5 of S3DIS and validation sets of ScanNet and nuScenes.}
    \small
    \resizebox{\linewidth}{!}{\begin{tabular}{l|cc|cc}
    \toprule
    Methods    & S3DIS      & nuScenes     & ScanNet & nuScenes \\ \midrule
    SPVCNN~\cite{SPVCNN2020ECCV} & \cellcolor{yellow!10}{}44.1 & \cellcolor{yellow!10}{}56.9 & \cellcolor{blue!10}{}46.8 & \cellcolor{blue!10}{}58.4 \\
    PPT~\cite{PPT2023ArXiv} & \cellcolor{yellow!10}{}63.9 & \cellcolor{yellow!10}{}65.4 & \cellcolor{blue!10}{}65.3 & \cellcolor{blue!10}{}65.8 \\
    GeoAuxNet        & \cellcolor{yellow!10}{}\textbf{68.4} & \cellcolor{yellow!10}{}\textbf{70.8} & \cellcolor{blue!10}{}\textbf{69.8} & \cellcolor{blue!10}{}\textbf{71.6}\\ \bottomrule
    \end{tabular}
    }
    
    \label{tab:additional results}
\end{table}

\subsection{Efficiency Analysis}
% To rigorously evaluate the effectiveness of our point networks and geometry pools, both designed for extracting local geometric features, we executed an ablation study by entirely removing the point branch. More precisely, voxel features are directly propagated to subsequent stage without being concatenated with features extracted from geometry pools via Geo-to-Occ Auxiliary. 
% As shown in Table~\ref{tab:efficiency}, we validate the efficiency of different models with latency. The speed up of GeoAuxNet over PointTransformer is $17.5\times$. Our method outperforms PPT by about 2\% in mIoU with $2.6\times$ measured speedup. This results further demonstrate the efficiency of GeoAuxNet.
% \begin{table}[h]
%     \centering
%     \caption{Efficiency analysis. We report the latency on per-processed data from S3DIS dataset.}
%     \begin{tabular}{l|c}
%     \toprule
%     Mehtods & Latency (ms / ins.) \\ \midrule
%     PointTransformer~\cite{PointTransformer2021ICCV} & 29.4 \\
%     PointTransformerV2~\cite{PointTransformerV22022NIPS} & 83.3 \\
%     MinkowskiNet~\cite{SparseUNet2019CVPR} & 1.1 \\
%     SPVCNN~\cite{SPVCNN2020ECCV} & 1.4 \\
%     PPT~\cite{PPT2023ArXiv} & 4.0 \\
%     GeeAuxNet & 1.7 \\ \bottomrule
%     \end{tabular}
    
%     \label{tab:efficiency}
% \end{table}

Auxiliary learning aims to improve the model performance on the primary task by exploiting beneficial information from auxiliary tasks, while auxiliary tasks can be removed during inference. Our idea is to design a voxel network for the primary task to maintain its efficiency, and a point network for the auxiliary task so that it provides geometric information and is removed during inference. While kNN limits the efficiency, during inference we only preserve the Geometry Pool and Geo-to-Occ Auxiliary modules without the point network and kNN. As shown in Table~\ref{tab:more efficiency}, we validate the efficiency of different models on various datasets.

\begin{table*}[h]
\centering
\caption{The inference time and throughput on data with a single NVIDIA A6000 GPU.}
\begin{tabular}{lc|ccc|ccc}
\toprule
\multirow{2}{*}{Method} & \multirow{2}{*}{Params.} & \multicolumn{3}{c|}{Inference Time (ms) \textcolor{red}{$\downarrow$}} & \multicolumn{3}{c}{Throughput (ins./sec.) \textcolor{green}{$\uparrow$}} \\ \cmidrule{3-8} 
                &        & ScanNet         & SemanticKITTI        & nuScenes        & ScanNet       & SemanticKITTI       & nuScenes       \\ \midrule
PointNet++~\cite{PointNet++2017NIPS}\    &1.0M          & 1987       & 2013      & 2195      & 96       & 880      & 300      \\
PT~\cite{PointTransformer2021ICCV}       &7.8M               & 5779       & 5814      & 6298      & 32       & 268      & 95       \\
PTv2~\cite{PointTransformerV22022NIPS}    &3.9M                & 24275      & 24834     & 27695     & 10       & 96       & 31       \\
MinkowskiNet~\cite{SparseUNet2019CVPR}   & 60.9M         & 237        & 245       & 275       & 728      & 31       & 2490      \\
SPVCNN~\cite{SPVCNN2020ECCV}    & 61.0M              & 246        & 244       & 284       & 550      & 2490     & 1922         \\
PPT~\cite{PPT2023ArXiv}       & 63.0M              & 402        & 407       & 471       & 210      & 1922     & 692         \\
GeoAuxNet       & 64.7M        & 267        & 269       & 303       & 462      & 692      & 1589         \\ \bottomrule
\end{tabular}
\label{tab:more efficiency}
\end{table*}

\section{Additional Visualization}
We provide more visualizations for MinkowskiNet~\cite{SparseUNet2019CVPR}, SPVCNN~\cite{SPVCNN2020ECCV}, PPT~\cite{PPT2023ArXiv} and GeoAuxNet in Figure~\ref{fig:visualization}. The limitation of learning sensor-specific information in MinkowskiNet leads to unsatisfactory performance on the joint training benchmark. 
PPT only utilize voxel representations, while the point branch in SPVCNN does not provide fine-grained geometric features.
The introduction of elaborate geometric information in GeoAuxNet preserves better detailed structures for point clouds from various sensors.

\section{Additional Discussion and Future Works}

Benefiting from extensive training data, universal models have achieved remarkable performance in natural language processing and 2D vision.
PPT~\cite{PPT2023ArXiv} studies cross-dataset learning in 3D vision which focuses on point clouds in different datasets from the same sensor. However, the domain gap between point clouds from different sensors still limits the university of 3D networks, which hampers the fusion and utilization of data from diverse sensors in practice. We propose GeoAuxNet to address this issue in an efficient way towards universal 3D representation learning.
However, high quality 3D data is limited compared with the large corpus and numerous images.
Therefore, our future researches will be undertaken to leverage text and 2D information for 3D universal models. Besides, more work will need to be done for the generation of scene-level 3D data.

% While GeoAuxNet shows encouraging performance on point clouds from different sensors with a uniform framework, it does not outperform the-state-of-art experts trained on each single dataset. 
% Universal models in NLP and 2D vision benefit from extensive training data. However, high quality 3D data is limited compared with the large corpus and numerous images. 
